# Supplementary material for: The Computational Complexity of Avoiding Strict Saddle Points in Constrained Optimization
Source: arXiv:2604.02285 source file (2026-11-04)
Supplement: Supplementary file 1 [file Appendix.tex]

\appendix
